# Supplementary material for: Monitoring Unmanned Aircraft: Specification, Integration, and Lessons-learned
Source: arXiv:2404.12035 source file (2024-04-18)
Supplement: Supplementary file 1 [file appendix.tex]

\newpage
\todo{sebas: do we have an appendix to add all of them or do you plan to have all of them in the paper?}
\section{RCC}
%\lstinputlisting{specification/single_rcc.lola}
%\lstinputlisting{specification/multiple_rcc.lola}

\section{DAA}

\section{Geofence}

\section{FPR}
